# Supplementary material for: Formation of human kinship structures depending on population size and cultural mutation rate
Source: arXiv:2407.10553 source file (2024-07-15)
Supplement: Supplementary file 1 [file clan_phys_PNAS_for_Supplementary_Information.pdf]

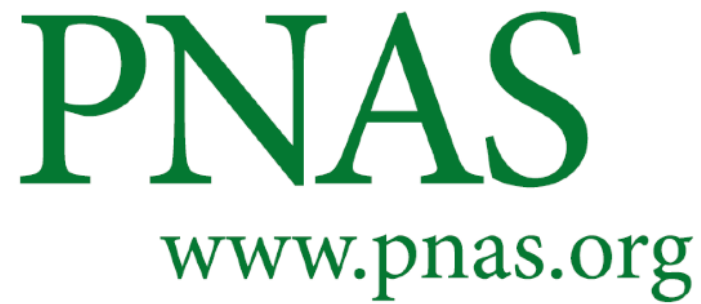

## **Supplementary Information for**

### **Formation of human kinship structures depending on population size and cultural mutation rate**

**Kenji Itao and Kunihiro Kaneko**

**Kunihiro Kaneko.**

**E-mail: [kaneko@complex.c.u-tokyo.ac.jp](mailto:kaneko@complex.c.u-tokyo.ac.jp)**

#### **This PDF file includes:**

Figs. S1 to S4

Table S1

References for SI reference citations

## Supplementary text

**Other possible mathematical formulations of the model.** In our model, the growth rate of each family  $i$  depends on the degree of preferredness:

$$D_p^i = \langle \exp(-(t_i - p_j)^2) \rangle_j / \langle \exp(-(t_i - t_j)^2) \rangle_j, \quad [1]$$

which is the ratio of the number of women who prefer someone like a man in the family  $i$  to the number of men like him.

There is another way to define the degree of preferredness by  $D'_p = \langle \exp(-(t_i - p_j)^2) / \langle \exp(-(t_k - p_j)^2) \rangle_k \rangle_j$ , instead of the current definition. These two definitions can be approximately equated as long as families form distinct clans in  $t - p$  space. Let us assume that the mismatch of mate clans'  $t$  and  $p$  is less than a small value  $\epsilon$ , whereas different clans are sufficiently distant in the  $t - p$  space. Then,

$$\begin{aligned} D'_p &= \left\langle \frac{\exp(-(t_i - p_j)^2)}{\langle \exp(-(t_k - p_j)^2) \rangle_k} \right\rangle_j \\ &= \left\langle \frac{\exp(-(t_i - p_j)^2) \times \hat{\delta}(|t_i - p_j| - \epsilon)}{\langle \exp(-(t_k - t_i + t_i - p_j)^2) \rangle_k} \right\rangle_j \\ &\simeq \left\langle \frac{\exp(-(t_i - p_j)^2) \times \hat{\delta}(|t_i - p_j| - \epsilon)}{\langle \exp(-(t_k - t_i + \epsilon)^2) \rangle_k} \right\rangle_j \\ &\simeq \frac{\langle \exp(-(t_i - p_j)^2) \rangle_j}{\langle \exp(-(t_i - t_k)^2) \rangle_k} \\ &= \frac{\langle \exp(-(t_i - p_j)^2) \rangle_j}{\langle \exp(-(t_i - t_j)^2) \rangle_j} = D_p, \end{aligned}$$

where  $\hat{\delta}(x)$  is 1 if  $x < 0$  and 0 otherwise. Note that  $\exp(-x^2)$  for  $x \gg \epsilon$  is almost 0, and the distances of  $t$  and  $p$  are sufficiently large for this approximation since different clans are sufficiently distant in  $t - p$  space. In addition, we have also simulated the model using  $D'_p$ . Then, the nearly identical structures evolve. In the current model, we use  $D_p$  because it is computationally efficient.

We have also simulated the models with the different forms of kinship interactions. First, we considered the dowry-type in-law cooperation where the density of cooperative friends for family  $i$  is given by

$$D_f^i = \langle \exp(-(t_i - t_j)^2) + (1 - \exp(-(t_i - t_j)^2)) \exp(-(t_i - p_j)^2) \rangle_j. \quad [2]$$

The results of this model are shown in Fig. S1. It demonstrates consistent results with the original model shown in Fig. 4.

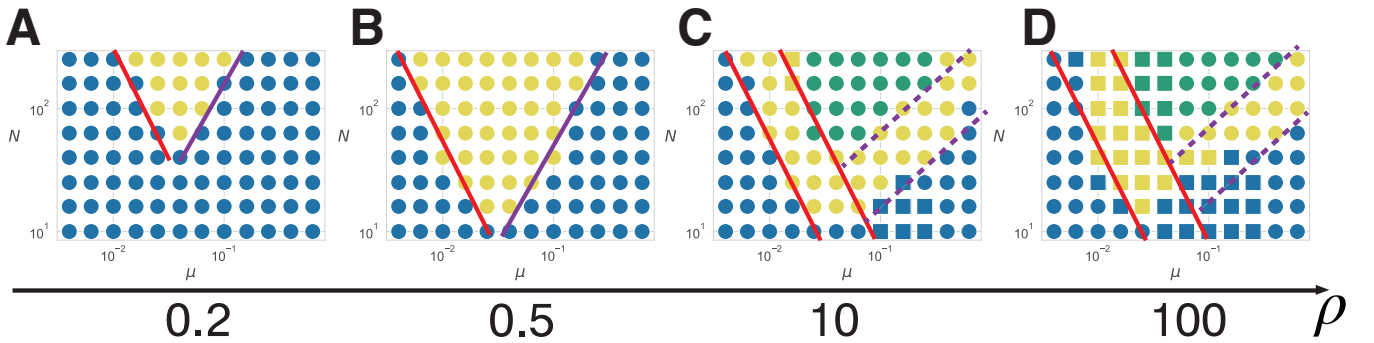

**Figure S1.** Phase diagram of the structures that evolve most frequently in 100 trials of simulation of the model variant with the dowry-type in-law cooperation, under the given parameters representing the number of families,  $N$ , and the mutation rate,  $\mu$ , for different  $\rho$  (comparable to Fig. 4). Colors indicate the marriage cycle length; endogamy,  $c_m = 1$  (blue), dual organization,  $c_m = 2$  (yellow), and generalized exchange,  $c_m \geq 3$  (green). Shapes show the number of tribes; a single tribal society,  $n_t = 1$  (circle), and multiple tribal society,  $n_t \geq 2$  (square). Red lines show the isoclines of  $N\mu^2$ . Purple lines in (A, B) show isoclines of  $\mu^2/N$  and the dashed lines in (C, D) show those of  $\mu/N$ .

Second, we considered the bidirectional in-law cooperation where the density of cooperative friends for family  $i$  is given by

$$D_f^i = \langle \min(\exp(-(t_i - t_j)^2), \exp(-(t_i - p_j)^2), \exp(-(p_i - t_j)^2)) \rangle_j. \quad [3]$$

This modification results in a slight difference. Due to the bidirectional in-law cooperation, each clan can have three cooperative clans at maximum (i.e., its own, the brides of its male members, and the grooms of its female members). Thus, structures with  $c_m = 3$  can evolve with  $\rho \leq 2$ . However, the scaling relationships of the phase boundaries are unchanged as shown in Fig. S2.

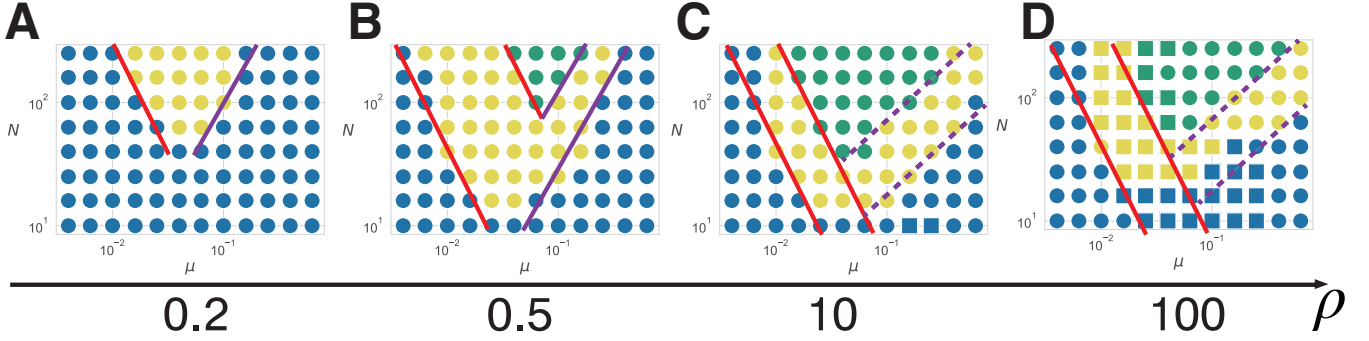

**Figure S2.** Phase diagram of the structures that evolve most frequently in 100 trials of simulation of the model variant with the bidirectional in-law cooperation, under the given parameters representing the number of families,  $N$ , and the mutation rate,  $\mu$ , for different  $\rho$  (comparable to Fig. 4). Colors indicate the marriage cycle length; endogamy,  $c_m = 1$  (blue), dual organization,  $c_m = 2$  (yellow), and generalized exchange,  $c_m \geq 3$  (green). Shapes show the number of tribes; a single tribal society,  $n_t = 1$  (circle), and multiple tribal society,  $n_t \geq 2$  (square). Red lines show the isoclines of  $N\mu^2$ . Purple lines in (A, B) show isoclines of  $\mu^2/N$  and the dashed lines in (C, D) show those of  $\mu/N$ . Due to the bidirectional in-law cooperation, each clan can have three cooperative clans at maximum (i.e., its own, the brides of its male members, and the grooms of its female members). Thus, structures with  $c_m = 3$  can evolve with  $\rho \leq 2$ .

Finally, we considered the mate preference by males in which the marriage possibility between men in family  $i$  and women in  $j$  is given by  $\exp(-(p_i - t_j)^2)$ . Accordingly, the settings are revised as follows. The possibility of a man in the family  $i$  finding a mate is given by the degree of preferredness:

$$D_p^i = \langle \exp(-(p_i - t_j)^2) \rangle_j / \langle \exp(-(p_i - p_j)^2) \rangle_j, \quad [4]$$

which is the ratio of the number of women who are preferred by someone like him to the number of men who have similar preferences as him. The density of cooperative friends for family  $i$  is given by

$$D_f^i = \langle \min(\exp(-(t_i - t_j)^2), \exp(-(t_i - p_j)^2), \exp(-(p_i - t_j)^2)) \rangle_j. \quad [5]$$

The density of competing rivals for family  $i$  is given by

$$D_r^i = \langle \exp(-(p_i - p_j)^2) \rangle_j. \quad [6]$$

The results are shown in Fig. S3. Although the structures with larger  $c_m$  or  $n_t$  evolve in the narrower regions, the scaling relationships of the phase boundaries are unchanged.

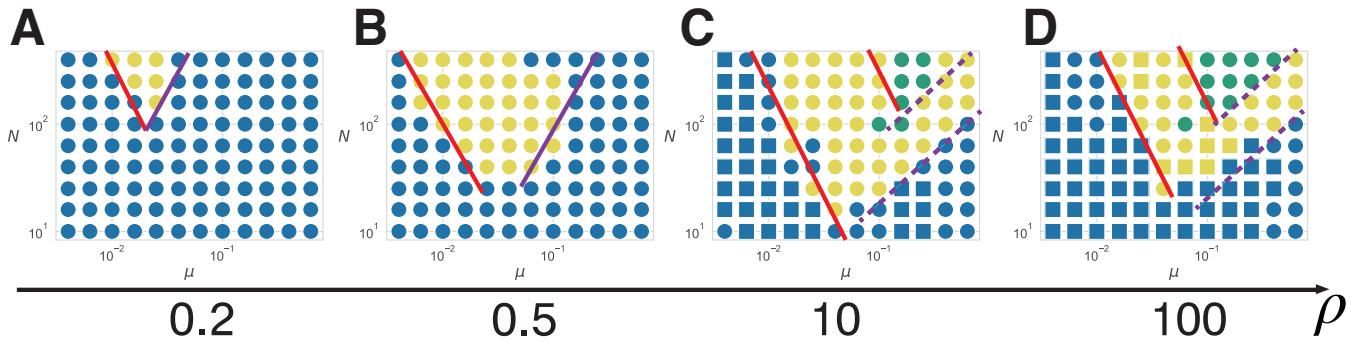

**Figure S3.** Phase diagram of the structures that evolve most frequently in 100 trials of simulation of the model variant with the mate preference by male, under the given parameters representing the number of families,  $N$ , and the mutation rate,  $\mu$ , for different  $\rho$  (comparable to Fig. 4). Colors indicate the marriage cycle length; endogamy,  $c_m = 1$  (blue), dual organization,  $c_m = 2$  (yellow), and generalized exchange,  $c_m \geq 3$  (green). Shapes show the number of tribes; a single tribal society,  $n_t = 1$  (circle), and multiple tribal society,  $n_t \geq 2$  (square). Red lines show the isoclines of  $N\mu^2$ . Purple lines in (A, B) show isoclines of  $\mu^2/N$  and the dashed lines in (C, D) show those of  $\mu/N$ .

**Empirical comparison.** We test the theoretical results by statistically analyzing the SCCS database (1, 2). The variables in the SCCS database describe various characteristics of a society, some of which can be used to identify kinship structure and estimate environmental parameters.

First, we classified each society's kinship structures by identifying the composition of clans and the marriage and descent rules between them by using the following variables in the SCCS database: SCCS70 *Descent*, SCCS221/223 *Largest patrilineal/matrilineal kin group*, SCCS222/224 *Largest patrilineal/matrilineal exogamous group*, and SCCS230 *Cousin marriages preferred*. See Table S1 for the identification procedure and the following detailed explanation of these variables. Of the 186 societies in the SCCS, their marriage cycle lengths are identified: the estimated values of  $c_m$  are 1 for 53 societies, 2 for 14, and  $\geq 3$  for 15. The identification of  $n_t$  was infeasible.

We then estimated population size  $N$ , mutation rate  $\mu$ , and the relative importance of avoiding rivalry versus having cooperation  $\rho$  from data. First,  $N$  is estimated by SCCS1122 *Log10 of total population*. Then,  $\mu$  is estimated by SCCS739/740 *Marriage arrangements (Male/Female)* and SCCS971/972 *Consent of the prospective wife/husband to marry*. Note that  $\mu$  denotes the similarity of traits and mating preferences between parents and children, and thus can be measured by the influence of parents in mate choice. Even when parents choose mates for their children, these selections may not replicate their own marital arrangements. However, it would be reasonable to expect greater intergenerational similarity in marriage patterns, especially when children follow or require parental approval for their mate choices rather than making autonomous decisions.) Finally,  $\rho$  is estimated by the ratio of the necessity of cooperation  $d_c$  and that of avoiding sexual rivalry  $d_m$ . The former  $d_c$  is estimated by using the variables on social unity (SCCS775 *Compliance of Individuals with Community Norms*, SCCS779 *Loyalty to the Society*, SCCS788 *Cross-cutting Ties*, and SCCS1737 *Extent of Burden Caused by Tribute Payments or Taxation*) and society-level conflict that requires immense cooperation within society (SCCS1770 *Attitude towards Physical Violence against Members of Other Ethnic Groups* and SCCS1772 *Hostility towards Other Ethnic Groups*). The latter  $d_m$  is estimated by using the variables on the extent of polygyny (SCCS861 *Standard Polygamy Code*), attitudes towards adultery (SCCS173 *Attitude toward Rape*, SCCS961 *Restrictions on Premarital Sex*, and SCCS963 *Restrictions and Extramarital Sex*), and intra-society conflict that can be caused by marital conflict (SCCS768 *Conflict between Communities of the Same Society*, SCCS773 *Internal Warfare between Communities of Same Society*, and SCCS782 *Acceptability of Violence toward Members of the Same Society*). See (3) for the discussion of the significance of these variables in estimating the parameter values.

To estimate  $\mu$ ,  $d_c$ , and  $d_m$ , we normalized the values of each variable to set the mean to 0 and the variance to 1. We changed the sign where necessary so that larger values of the variables corresponded to larger values of the parameters. For some societies, data were missing for some variables; however, we averaged the available values. We then normalized the estimated values to set the minimum to 0 and the maximum to 1. Then  $\rho$  is calculated as  $d_m/d_c$ .

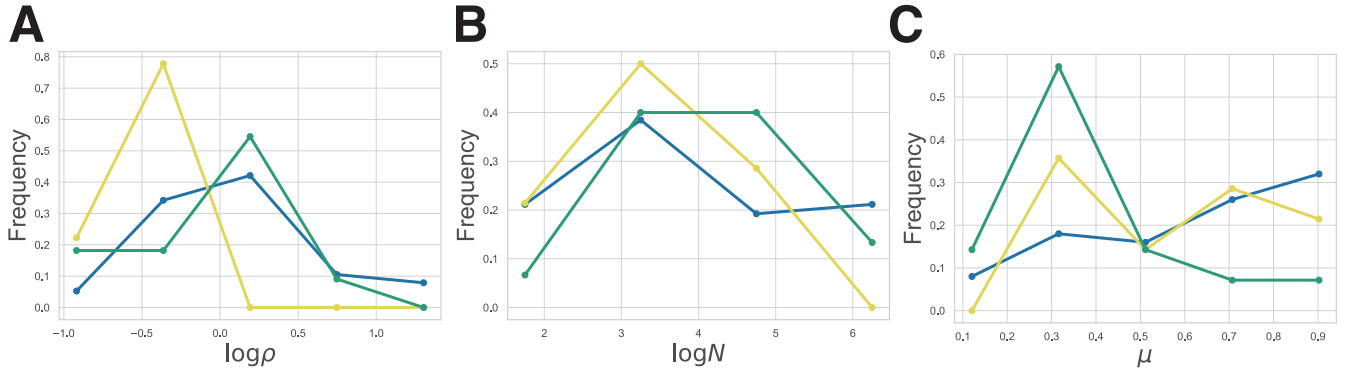

**Figure S4.** Empirical dependence of kinship structures on (A) the relative importance of avoiding rivalry versus having cooperation  $\rho$  (B) population size  $N$  and (C) mutation rate  $\mu$  by using the SCCS data. Colors indicate the marriage cycle length; endogamy,  $c_m = 1$  (blue), dual organization,  $c_m = 2$  (yellow), and generalized exchange,  $c_m \geq 3$  (green).

Fig. S4 shows the empirical dependence of kinship structures on the relative importance of avoiding rivalry versus having cooperation  $\rho$ , population size  $N$ , and mutation rate  $\mu$ . Consistent with the theoretical results,  $c_m$  is larger when  $\rho$  and  $N$  are larger, and  $\mu$  takes an intermediate value. Structures with  $c_m = 2$  are mainly observed with small  $\rho$ . The mean and standard variation of the estimated values are  $\log \rho = 0.08 \pm 0.57$ ,  $\mu = 0.59 \pm 0.25$  and  $\log N = 3.8 \pm 1.6$  for  $c_m = 1$ ,  $\log \rho = -0.47 \pm 0.30$ ,  $\mu = 0.56 \pm 0.25$  and  $\log N = 3.2 \pm 1.2$  for  $c_m = 2$ , and  $\log \rho = -0.03 \pm 0.52$ ,  $\mu = 0.35 \pm 0.21$  and  $\log N = 4.1 \pm 1.4$  for  $c_m \geq 3$ . Note that the estimates of the parameter values have large errors and the sample size is limited. Thus, it is difficult to empirically verify scaling relationships against  $N$  and  $\mu$ .

## Supplementary table

Table S1. Identification of kinship structures. We determined kinship structures by identifying the composition of clans, and the descent and marriage rules between them. Here, we used the variables for the largest kin groups (SCCS221 and SCCS223), exogamous units (SCCS222 and SCCS224), descent systems (SCCS70), and cousin preferences for mates (SCCS230). Exclusive conditions for identifying the same class are described in different rows. Largest kin groups refer to the presence of kin groups,  $SCCS221$  (or  $SCCS223$ )  $< 3$  indicates the absence of patrilineal (or matrilineal) kin groups and  $\geq 3$  indicates its presence. Exogamous units refer to the groups in which marriage is prohibited, i.e., clans.  $SCCS222$  (or  $SCCS224$ )  $= 1$  indicates patrilineal (or matrilineal) endogamy and  $\geq 2$  indicates patrilineal (or matrilineal) exogamy. The descent system refers to trait inheritance, either patrilineal, matrilineal, or double descent.  $SCCS70 = 1$  indicates matrilineal, 2 indicates double, and 3 indicates patrilineal descent system. Marriage rules between clans can be provided by cousin marriage preferences. Then, clan endogamy,  $c_m = 1$ , has no exogamous units (specifically, none larger than cohabitant groups). The dual organization,  $c_m = 2$ , is characterized by marriage prohibition within patrilineal (or matrilineal) moieties, patrilineal (or matrilineal) descent systems, and mating preference for symmetrical cross-cousins. Generalized exchange,  $c_m \geq 3$ , is characterized by marriage prohibition within patrilineal (or matrilineal) clans, patrilineal (or matrilineal) descent system, and mating preference for the mother's brother's daughter (or father's sister's daughter).

| $c_m$    | Explanation                                                  | Criterion                                      |
|----------|--------------------------------------------------------------|------------------------------------------------|
| 1        | No kin groups                                                | $SCCS221 < 3$ and $SCCS223 < 3$                |
| 2        | Patrilineal moiety exogamy                                   | $SCCS222 = 6$ and $SCCS224 = 1$                |
|          | Matrilineal moiety exogamy                                   | $SCCS222 = 1$ and $SCCS224 = 6$                |
|          | Patrilineal descent with symmetrical cross-cousin preference | $SCCS70 = 3$ , $SCCS222 > 1$ and $SCCS230 = 1$ |
|          | Matrilineal descent with symmetrical cross-cousin preference | $SCCS70 = 1$ , $SCCS224 > 1$ and $SCCS230 = 1$ |
| $\geq 3$ | Patrilineal descent with MoBrDa preference                   | $SCCS70 = 3$ and $SCCS230 = 2$                 |
|          | Patrilineal exogamy with MoBrDa preference                   | $SCCS222 > 1$ and $SCCS230 = 2$                |
|          | Matrilineal descent with FaSiDa preference                   | $SCCS70 = 3$ and $SCCS230 = 3$                 |
|          | Matrilineal exogamy with FaSiDa preference                   | $SCCS224 > 1$ and $SCCS230 = 3$                |

## Detailed explanation of SCCS variables

The values of SCCS variables are explained below (1, 2).

### SCCS70 Descent - Membership in Corporate Kinship Groups

1. Matrilineal—through female line, 2. Double descent—separate groups through male and female lines, 3. Patrilineal—through male line, 4. Ambilineal—through one parent in each generation, and 5. Bilateral—not a corporate kin group.

### SCCS173 Rape

1. Accepted/ignored, 2. Ridiculed, 3. Mildly disapproved, and 4. Strongly disapproved.

### SCCS221 Largest patrilineal kin group

1. None, 2. Exogamy only, 3. Lineages, 4. Sibs, 5. Phratries, and 6. Moieties.

### SCCS222 Largest patrilineal exogamous group

1. No exogamy, 2. Extended taboo, 3. Lineages, 4. Sibs, 5. Phratries, and 6. Moieties.

### SCCS223 Largest matrilineal kin group

1. None, 2. Exogamy only, 3. Lineages, 4. Sibs, 5. Phratries, and 6. Moieties.

### SCCS224 Largest matrilineal exogamous group

1. No exogamy, 2. Extended taboo, 3. Lineages, 4. Sibs, 5. Phratries, and 6. Moieties.

### SCCS230 Cousin marriages preferred: subtypes [Note, identical to EA026]

1. Symmetrical cross-cousin, 2. Mother's brother's daughter, 3. Father's sister's daughter, 4. Father's brother's daughter, 5. Second cousin, and 9. None preferred.

### SCCS739 Marriage Arrangements

1. Individual selects partner, 2. Individual selects/courts partner autonomously but approval necessary or highly desirable, 3. Individual suggests partner to parents/others: proceeds if approved, 4. Individual choice and arranged marriages are alternatives, 5. Parents choose partner: individual can object, and 6. Parents select partner

### SCCS740 Marriage Arrangements (Female)

1. Individual selects partner, 2. Individual selects/courts partner autonomously but approval necessary or highly desirable, 3. Individual suggests partner to parents/others: proceeds if approved, 4. Individual choice and arranged marriages are alternatives, 5. Parents choose partner: individual can object, and 6. Parents select partner

### SCCS773 (No) Internal Warfare (between Communities of Same Society)

1. Frequent, occurring at least yearly, 2. Common, at least every five years, 3. Occasional, at least every generation, and 4. Rare or never.

**SCCS775 (Low) Compliance of Individuals with Community Norms and Decisions**

1. High, 2. Moderate, and 3. Highly Variable.

**SCCS779 (Low) Loyalty to the Wider Society (in Some Cases Indistinguishable from the Local Community)**

1. Especially high, 2. High, 3. Moderate, and 4. Low.

**SCCS782 (Un) Acceptability of Violence toward Members of the Same Society, but outside the Local Community**

1. Valued, 2. Acceptable, 3. Tolerated, and 4. Disapproved.

**SCCS788 Cross-cutting Ties: Extent to Which Individuals Living in Different Communities of the Same Society Linked Together in Politically Relevant Ways**

1. No politically relevant links, formal organizations, or strong informal obligations which extend beyond the local community, 2. Some politically relevant ties, but wider society divided into some discrete groups not linked through cross-cutting ties, 3. Cross-cutting ties link individuals throughout the society, cutting across territorial groups in one or more ways.

**SCCS861 Standard Polygamy Code**

0. Polyandry, 1. Monogamy prescribed, 2. Monogamy preferred but exceptional cases of polygyny, 3. Limited polygyny < 20 pct of married males, and 4. Full polygyny 20 pct or more of married males.

**SCCS961 Restrictions on Premarital Sex**

1. It is permitted for both sexes, 2. It is permitted for both sexes, but in limited contexts, e.g., with prostitutes or as part of a ceremony, 3. It is permitted and not punished unless pregnancy results, 4. It is permitted for males but not for females, 5. Premarital relations are disapproved but infrequent, 6. Insistence on virginity for the women. There is no information on restrictions on the male, and 7. Premarital relations are strongly disapproved and rare.

**SCCS963 Restrictions and Extramarital Sex**

1. Permitted for both husband and wife, 2. Permitted for both but only in limited contexts (e.g., with particular relatives of the spouse, ceremonial license), 3. Permitted and not punished unless pregnancy results, 4. Permitted for the husband but not for the wife, 5. Weakly prohibited (e.g., frequent violations or weak punishment), and 6. Strongly prohibited (e.g., occurs rarely or severe punishment).

**SCCS971 How Necessary Is the Consent of the Prospective Wife for Marriage Arrangements to Proceed**

1. Prospective spouse's consent is necessary, 2. The prospective spouse is consulted, and 3. The prospective spouse is not consulted.

**SCCS972 How Necessary Is the Consent of the Prospective Husband for Marriage Arrangements to Proceed**

1. Prospective spouse's consent is necessary, 2. The prospective spouse is consulted, and 3. The prospective spouse is not consulted.

**SCCS1122 Log10 of Total Population**

1. 10-99, 2. 100-999, 3. 1,000-9,999, 4. 10,000-99,999, 5. 100,000-999,999, 6. 1,000,000-9,999,999, 7. 10,000,000-99,999,999, and 8. 100,000,000-999,999,999.

**SCCS1737 Extent of Burden Caused by Tribute Payments or Taxation**

20. Sporadic taxation or request for tribute, 21. Sporadic exactions are reported not to be burdensome, 22. Sporadic exactions are reported to be burdensome, 30. Regular taxation or request for tribute, 31. Regular exactions are reported not to be burdensome, and 32. Regular exactions are reported to be burdensome.

**SCCS1770 Attitude towards Physical Violence against Members of Other Ethnic Groups**

10. Physical violence outside of ethnic group is rejected, 11. Physical violence outside of ethnic group is rejected because of military inferiority or cowardice, 20. Physical violence is tolerated or accepted—specification of the enemies is absent, 21. Physical violence is tolerated or accepted but not against the majority of other ethnic groups, 22. Physical violence is tolerated or accepted against the majority of other ethnic groups, 30. Physical violence is appreciated—no further specification against whom, 31. Physical violence is appreciated but not against the majority of other ethnic groups, and 32. physical violence is appreciated against the majority of other ethnic groups.

**SCCS1772 Hostility towards Other Ethnic Groups**

10. No or negligible hostility, 20. Weak degree of hostility, 30. Moderate degree of hostility, 31. Moderate degree of hostility only directed against certain other ethnic groups, 32. Moderate degree of hostility directed against almost all other ethnic groups, 40. High degree of hostility, 41. High degree of hostility only directed against certain other ethnic groups, and 42. High degree of hostility directed against almost all other ethnic groups.

## References

1. GP Murdock, DR White, Standard cross-cultural sample. *Ethnology* **8**, 329–369 (1969).
2. KR Kirby, et al., D-place: A global database of cultural, linguistic and environmental diversity. *PloS one* **11**, e0158391 (2016).
3. K Itao, K Kaneko, Emergence of kinship structures and descent systems: multi-level evolutionary simulation and empirical data analysis. *Proc. Royal Soc. B* **289**, 20212641 (2022).
